# Supplementary material for: On-and-off chip cooling of a Coulomb blockade thermometer down to 2.8 mK
Source: arXiv:1708.09491 ancillary file (2017-08-30)
Supplement: Supplementary file 1 [file SOM.pdf]

Supplementary Material

# On-and-off chip cooling of a Coulomb blockade thermometer down to 2.8 mK

M. Palma,[1, a)] C. P. Scheller,[1, a)] D. Maradan,[1, 2] A. V. Feshchenko,[3] M. Meschke,[3] and D. M. Zumbühl[1, b)]

[1)] *Department of Physics, University of Basel, Klingelbergstrasse 82, CH-4056 Basel, Switzerland*

[2)] *Physikalisch-Technische Bundesanstalt (PTB), Bundesallee 100, 38116 Braunschweig, Germany*

[3)] *Low Temperature Laboratory, Department of Applied Physics, Aalto University, P.O. Box 13500, FI-00076 AALTO, Finland*

(Dated: 30 August 2017)

---

[a)] These authors contributed equally to this work.

[b)] dominik.zumbuhl@unibas.ch

## I. SAMPLE FABRICATION AND MODE OF OPERATION

The device is fabricated on top of a silicon wafer with an insulating $SiO_2$ layer in two steps using electron-beam lithography. In the first lithography step, a ground plane is created that consists of 50 nm of Cu and is covered by a 100 nm of $Al_2O_3$ insulator, grown by atomic layer deposition. In the second lithography step, a 40 nm thick Al bottom electrode is evaporated and subsequently *in-situ* thermally oxidized. After the oxidation, a 40 nm thick top Al electrode is evaporated under a different tilt angle (two-angle shadow mask evaporation), thereby forming an Al-$AlO_x$-Al tunnel junction of $1\,\mu m^2$ area. Finally, the top Al electrode is overgrown with a 200 nm thick Cu layer of the same geometry and tilt angle. Hence, the Cu layer of the top electrode makes available a large reservoir of nuclear spins that may be used for adiabatic nuclear demagnetization (AND) experiments.

Metallic Coulomb blockade thermometers (CBTs) can be operated in two different modes, either as a primary thermometer, where the electronic temperature is inferred from the full bias dependence (or simply the full width at half maximum of the zero bias conductance dip, when neglecting ohmic heating effects), or as secondary thermometer. In the latter mode of operation, the relative conductance dip size $\delta g = (g_T - g_0)/g_T$ can be used as a measure of temperature after pre-calibration at high temperature where the device is at equilibrium with the Cu plates, $T_{Cu} = T_{CBT}$. Here, $g_0$ and $g_T$ denote the conductance at zero and high bias, respectively. Figure S1(a,b,c) shows bias traces in red color, recorded at $T_{Cu} = 60\,mK$, $T_{Cu} = 20\,mK$, and $T_{Cu} = 10\,mK$, respectively. In addition, the zero bias conductance traces (black curves), measured as a function of time right after the respective bias traces, are shown. At high temperature $T_{Cu} > 15\,mK$, the minimum conductance from bias traces agrees very well with $g_0$ measured as a function of time at effectively zero bias, see Fig. S1(a,b). However, a clear deviation is observed at low temperature e.g. $T_{Cu} = 10\,mK$, where the conductance $g_0$ drops over a time scale of roughly ten minutes and saturates well below the minimum value obtained from the bias scan, as seen in Fig. S1(c). This indicates overheating of the device at finite bias. The thermal relaxation time is very long and increases sharply at lower temperatures. Thus, there is not nearly enough time for adequate equilibration of the zero bias point taken during the scan. Scanning at sufficiently slow speed would consume hours or longer and is therefore not practical. In addition, while some steady state situation may be reached eventually after a long time, this may still be in

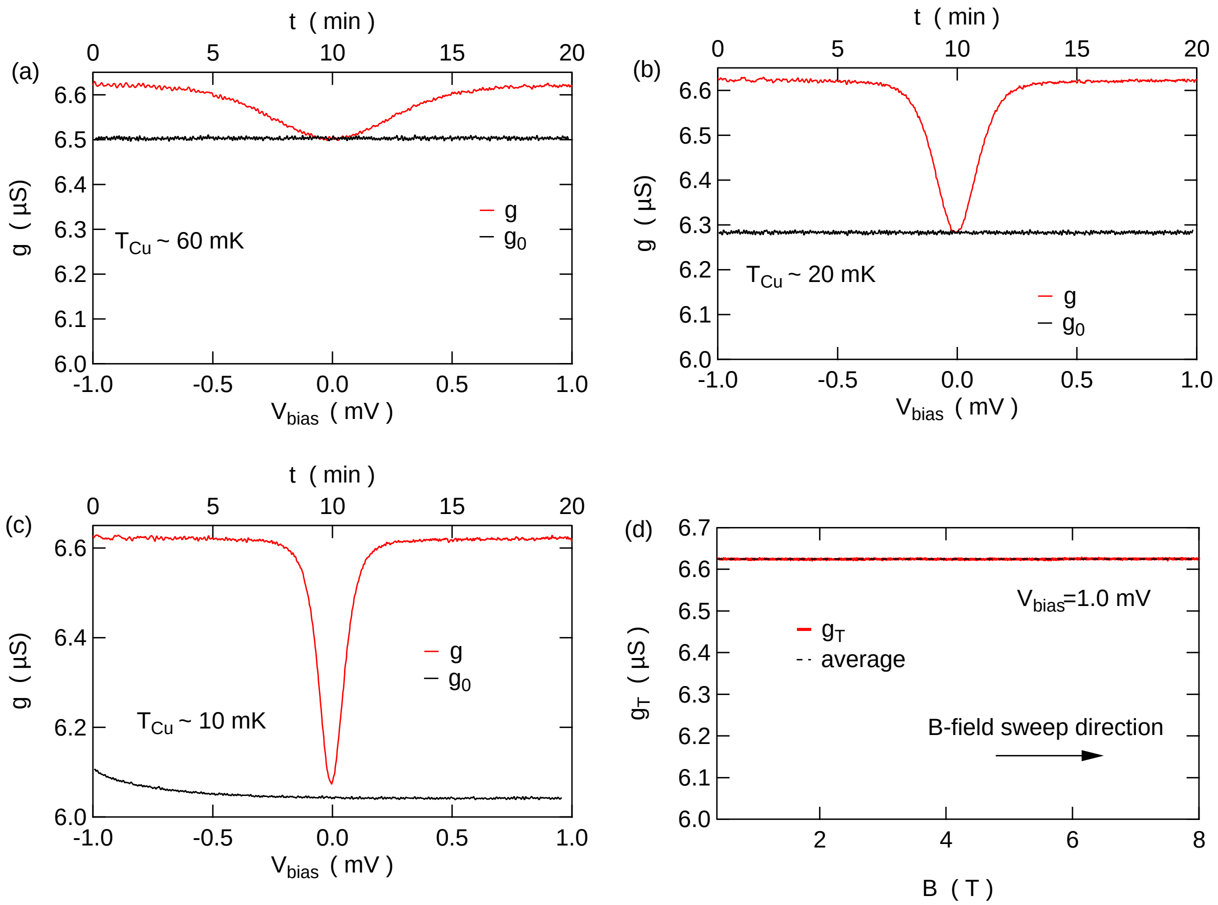


FIG. S1. (a-c) Differential conductance as a function of voltage bias (red data), shown for different temperatures as indicated. In addition, the differential conductance measured at zero bias as a function of time (data taken immediately after the corresponding bias scan) is shown in black, plotted versus the upper axis. (d) High bias ($V_{\mathrm{bias}} = 1\,\mathrm{mV}$) magneto-conductance $g_{\mathrm{T}}$ and its average value are shown in red and black, respectively. No magnetic field dependence is observed.

an overheated state when not at zero bias. We therefore measure exclusively at zero bias to avoid overheating and use the relative conductance dip size after pre-calibration to measure temperature.

Staying very close to zero bias within a narrow window of tolerance over long periods of time e.g. hours or days is not trivial. Commercially available instruments usually have significant drift of $\pm 10\,\mu\mathrm{V}$ or more of the voltage emanating from the amplifier input (input voltage), thus changing the bias voltage. To avoid these problems, we have built a low noise, high stability current preamplifier which keeps its input voltage stable within $\pm 0.15\mu\mathrm{V/K}$, see Ref. 1 for details. This eliminates the need for any cumbersome corrections or external

feedback to keep the bias very close to zero voltage.

In addition, applying a high bias to the CBT quickly destroys any previous nuclear heat capacity and AND cooling, thus giving us yet another reason to only monitor the zero bias conductance, particularly during demagnetization and warm up in the main text. For reliable temperature extraction, we need to assume that the high bias tunneling conductance value $g_T$ (needed for calculation of the relative conductance dip size $\delta g = 1 - g_0/g_T$ ) is independent of magnetic field. In order to test this assumption, the magneto-conductance at $V_{\text{bias}} = 1\,\text{mV}$ is shown in Fig. S1(d). Indeed, the high bias conductance is observed to be B-field independent to within our measurement error. This guarantees that the sole measurement of the zero bias conductance is a reliable and simple thermometer.

## II. EXPERIMENTAL SETUP

Efficient thermalization and filtering of the leads from room temperature down to the mixing chamber (MC) is required in order to sufficiently suppress microwave radiation. The leads consist of thermocoaxes[2], thermalized to the different temperature stages of the dilution refrigerator, followed by low resistance home-built Ag-epoxy microwave filters[3] and standard 2-pole RC-filters with 45 kHz cut-off frequency. After the filtering stages, the leads are fed through the mixing chamber, where they are efficiently thermalized with the $^3\text{He}-^4\text{He}$ mixture by means of Ag-sinters[4,5]. They continue as massive, annealed Ag-wires and finally, each wire is spot-welded to its own Cu plate. In order to thermally decouple the Cu pieces from the mixing chamber during AND, the silver wires are fused to Aluminum heat switches[6]. The temperature of the Cu pieces is measured with a magnetic field fluctuation thermometer[7–9], connected to a SQUID amplifier[10]. This thermometer performs an inductive read-out of the thermal currents inside an annealed Ag-wire[11,12], which is well thermally coupled to one of the Cu pieces.

## III. WARM UP WITH HEAT APPLIED TO THE CU PLATES

In the main text, the warm up of the CBT was monitored for the first 20 hours after nuclear demagnetization. After roughly 8 hours the CBT temperature increased and saturated at 7.5 mK electron temperature, while the Cu plate temperature $T_{\text{Cu}}$ is almost unchanged

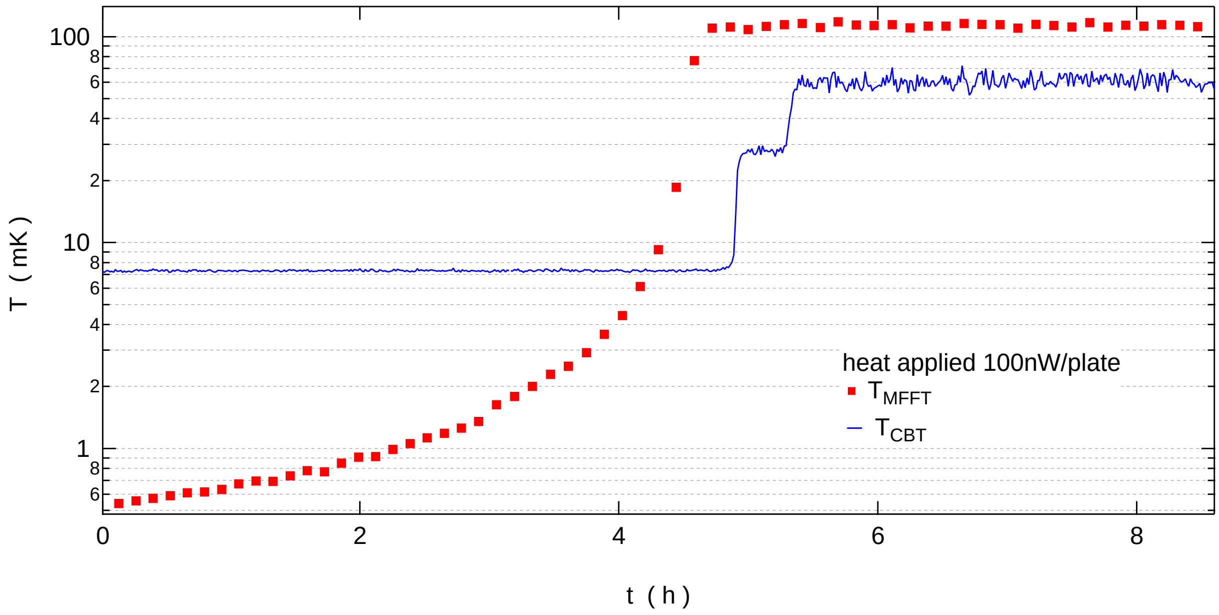


FIG. S2. Warm up curves $T_{\mathrm{CBT}}$ and $T_{\mathrm{Cu}}$ for the CBT and the Cu plate, respectively, upon applying an external heat load of 100 nW/plate (for 3 different Cu plates).

during this period. Here, we discuss the further warm up behavior of the CBT, when the Cu plates themselves start to warm up. In order to speed up this process, a heat load is applied to three Cu plates (100 nW/plate). One of these plates carries the MFFT thermometer, used to measure the Cu plate temperature, and serves at the same time as one of the leads for the CBT. The other two plates are left without additional function.

The Cu plate reacts immediately to the large external heat load, rises above 1 mK after a bit more than 2 hours, and finally heats above the CBT temperature after more than 4 hours. About half an hour after this crossing of temperatures, and roughly ten minutes after the complete Cu plate warm up, $T_{\mathrm{CBT}}$ jumps abruptly up to $\approx 30$ mK, see first step in $T_{\mathrm{CBT}}$ in Fig. S4. Before that, the CBT temperature remains constant for the first $\approx 5$ hours, indicating strong thermal decoupling of those systems. After waiting another $\approx 15$ minutes at $\approx 30$ mK, a second step is observed, raising the CBT temperature to $\approx 60$ mK. The second step is possibly due to a delayed warm up of the Cu plate hosting the CBT, which is not directly heated.

## IV. HIGH CHARGING ENERGY CBT

Here, we compare on-and-off chip magnetic cooling of a second CBT device with higher charging energy ($E_c = 17.2\,\mathrm{mK}$ instead of $E_c = 6.5\,\mathrm{mK}$), different number of junctions (64 instead of 32 junctions) and much smaller CBT island volume (300 $\mu\mathrm{m}^3$ instead of $42,000$ $\mu\mathrm{m}^3$) compared to the one shown in the main text, see Fig. S3(b). As described in the main text, this can deliver some important clues about the origin of the heat leak. Both CBTs are mounted in the same Cu box (Faraday cage), use the same microwave filters, and are measured in two different cool-downs. While the relative conductance dip size in Fig. S3(a,b) clearly reflects the differing charging energies, the extracted electron tem-

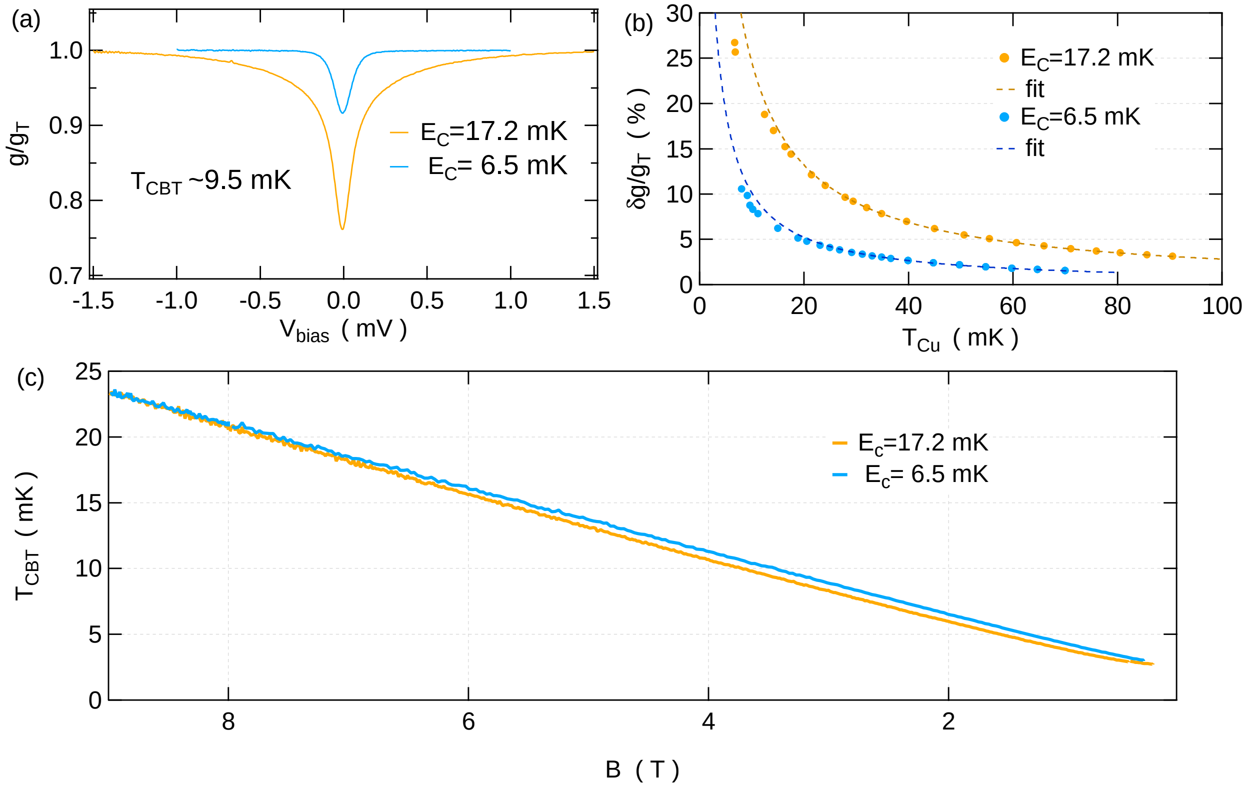


FIG. S3. (a) Differential conductance as a function of voltage bias, normalized to the high bias value, shown for 2 devices with different charging energy, and recorded at base temperature of the refrigerator. (b) Relative conductance dip size versus temperature for the two devices in (a). Dashed traces are curve fits to Eq.1 from the main text, used to extract the charging energy. (c) CBT temperature for both devices, measured as a function of applied magnetic field during the adiabatic nuclear demagnetization process.

perature is the same in both cases, as expected. This holds also for the adiabatic nuclear demagnetization process, giving a final temperature of $\approx$ 2.5 mK after demagnetization, close to the 2.8 mK reported in the main text for the low charging energy device. However, while the $E_c = 17.2$ mK device is more accurate for the high temperature regime, precise temperature extraction (to within 10 %) is only guaranteed down to roughly 5 mK[13,14]. Nonetheless, the demagnetization behavior of the two devices are consistent, thus giving additional confirmation for the low temperature results in the main text.

## V. VIBRATIONS AND ELECTRICAL NOISE

The large precooling temperature of the CBT (see main article) and the reduced efficiency during the adiabatic nuclear demagnetization process are the two main limiting factors for reaching lower temperatures. In this section, we discuss vibration induced eddy current heating as a possible cause for both factors. In order to investigate this scenario, the voltage across the CBT is measured during 50 s using a fast DAQ with the sample mounted in perpendicular configuration (in contrast to all other data). Fig. S4(a,b) show the Fast Fourier Transform (FFT) for such time traces, recorded at magnetic fields ranging from 80 mT up to 8 T.

The FFT shows frequency bands with varying noise level. In particular, up to 20 Hz, the level is rather low (note that lock-in measurements are done at 7 Hz) while it increases significantly above 20 Hz and has a pronounced peak structure around 140 Hz (see integrated noise at 4 T in Fig. S4(c)). A zoom in around 140 Hz shows a clear substructure with very sharp peaks, separated exactly by the pulse tube frequency of 1.4 Hz. This suggests that around 140 Hz the nuclear stage vibrates at an eigenfrequency and is driven by the slow vibrations of the pulse tube. As the field is changing, some of these vibration noise peaks seem to grow while others become weaker. We note that at low field <0.1 T, the overall noise integrated up to 1 MHz is about 1 $\mu$Vrms. At higher fields this increases by about an order of magnitude with a broad peak around 2-3 T. In addition to vibration induced noise, also the omnipresent 50 Hz noise peak (and its multiples, e.g. at 150 Hz) are clearly seen in the FFT spectrum. The electrical noise at 150 Hz shows small frequency variations, in contrast to the vibration induced peaks.

In conclusion, Fig. S4 suggests that there is a significant level of vibrations in the present

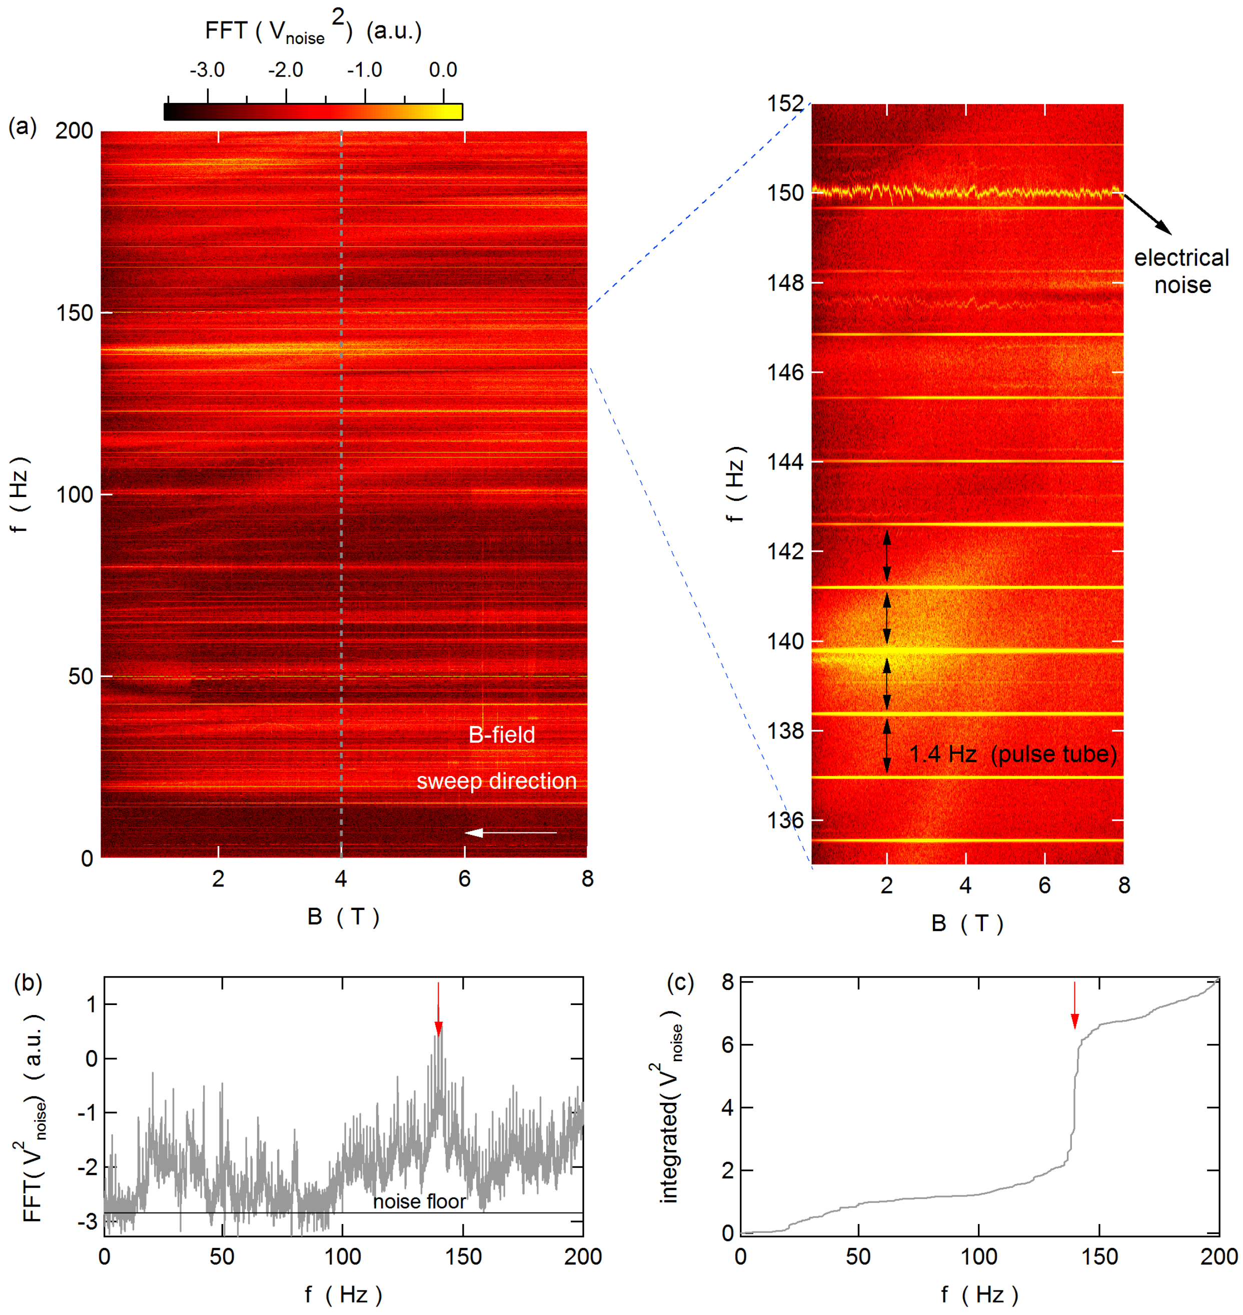


FIG. S4. (a) Logarithm of the absolute value of the noise spectrum as function of the frequency and magnetic field. A zoom-in of the frequency range between 135 Hz and 152 Hz is shown on the right hand side. (b) Vertical cut of (a) at 4 T. (c) Integrated noise of the spectrum shown in (b). A red arrow indicates a large increase in the noise level around 140 Hz.

system, which displaces the sample periodically from the center of the solenoid and therefore results in a time-dependent magnetic field. The resulting vibration induced eddy current heating may present one of the limiting factors for the current measurement and will be

addressed in future experiments.

## REFERENCES


[1]Basel Electronics Lab, Physics Departement, University of Basel, Switzerland.

[2]A. B. Zorin, "The thermocoax cable as the microwave frequency filter for single electron circuits," Rev. Sci. Instrum. **66**, 4296–4300 (1995).

[3]C. P. Scheller, S. Heizmann, K. Bedner, D. Giss, M. Meschke, D. M. Zumbühl, J. D. Zimmerman, and A. C. Gossard, "Silver-epoxy microwave filters and thermalizers for millikelvin experiments," Appl. Phys. Lett. **104**, 211106 (2014).

[4]A. C. Clark, K. K. Schwarzwälder, T. Bandi, D. Maradan, and D. M. Zumbühl, "Method for cooling nanostructures to microkelvin temperatures," Rev. Sci. Instrum. **81**, 103904 (2010).

[5]M. Palma, D. Maradan, L. Casparis, T.-M. Liu, F. N. M. Froning, and D. M. Zumbühl, "Magnetic cooling for microkelvin nanoelectronics on a cryofree platform," Rev. Sci. Instrum. **88**, 043902 (2017).

[6]N. Lawson, "A simple heat switch for use at millikelvin temperatures," Cryogenics **22**, 667 – 668 (1982).

[7]D. Rothfuss, A. Reiser, A. Fleischmann, and C. Enss, "Noise thermometry at ultra low temperatures," Appl. Phys. Lett. **103**, 052605 (2013).

[8]J. Engert, D. Heyer, J. Beyer, and H. J. Barthelmess, "Noise thermometry at low temperatures: Mfft measurements between 1.6 k and 1 mk," J. Phys. Conf. Ser. **400** (2012).

[9]J. Beyer, D. Drung, A. Kirste, J. Engert, A. Netsch, A. Fleischmann, and C. Enss, "A magnetic-field-fluctuation thermometer for the mk range based on squid-magnetometry," IEEE Trans. Appl. Supercond. **17**, 760–763 (2007).

[10]1-stage current sensor C4L1W DC-SQUID, Magnicon GmbH, Hamburg, Germany.

[11]H. Nyquist, "Thermal agitation of electric charge in conductors," Phys. Rev. **32**, 110–113 (1928).

[12]J. B. Johnson, "Thermal agitation of electricity in conductors," Phys. Rev. **32**, 97–109 (1928).

[13]M. Meschke, J. P. Pekola, F. Gay, R. E. Rapp, and H. Godfrin, "Electron thermalization in metallic islands probed by coulomb blockade thermometry," J. Low Temp. Phys. **134**,

1119–1143 (2004).

[14] A. V. Feshchenko, M. Meschke, D. Gunnarsson, M. Prunnila, L. Roschier, J. S. Penttilä, and J. P. Pekola, "Primary thermometry in the intermediate coulomb blockade regime," J. Low Temp. Phys. **173**, 36–44 (2013).
